# Supplementary material for: Problems with Cosine as a Measure of Embedding Similarity for High Frequency Words
Source: arXiv:2205.05092 source file (2022-05-10)
Supplement: Supplementary file 1 [file extra.tex]

Here we ask, are there differences in how much context is embedded into each word and does this vary with frequency? We design an experiment called, \textbf{contextual retrieval}, where the task is to identify a word's original context when given only the word's embedding. We embed words in identical contexts using thirty random sentences and inserting a random word at a random index (e.g. Sentence \#1: "Her insurance was \_\_\_\_ \$1000"). For training, we insert BERT's mask token ("[MASK]") at the random index and create embeddings of the masked token in all thirty different contexts. The word embeddings are the training data and the labels are the sentence numbers corresponding to the context the word embedding was created with. When inserting a set of five hundred random words into the articial dataset, a simple logistic regression model achieves an average accuracy of 97\%.

\begin{figure}[h]
    \centering
    \vspace{-0.5 em}
     \includegraphics[width=.48\textwidth]{Images/Findings1/ContextualRetrivalResults.png}
     \vspace{-1 em}
     \caption{The error rate is negatively correlated with the frequency of the word in BERT's original training data.}
     \label{fig: contextual retrieval}
     \vspace{-0.5 em}
\end{figure}

We find that it is easy to retrieve the original context of a word given its word embedding and that there is a correlation (Pearson's $r$: 0.36, \textit{p} < 0.001) between the log(frequency) of the word in BERT's original training data and the performance of the word on this task. We see that words with lower frequency (< 1,000 occurrences in training data) have a 4.5\% error rate whereas higher frequency words (> 100,000 occurrences in training data), have less than a 0.07\% error rate (see figure \ref{fig: contextual retrieval}).

This experiment highlights the discrepancies in the amount of context that is embedded and how it varies with a word's training data frequency. It supports our hypothesis that frequency-based distortions are partly due to how the model embeds high and low frequency words differently.
